# Supplementary material for: Surface Wave Transmission Line Theory for Single and Many Wire Systems
Source: arXiv:2103.10821 source file (2021-03-19)
Supplement: Supplementary file 1 [file SupplementaryMaterial.pdf]

# Supplementary Material: Surface Wave Transmission Line Theory for Single and Many Wire Systems

Tobias Schaich, Daniel Molnar, Anas Al Rawi, Mike Payne

February 26, 2021

## 1 Photos of Experimental Setup

Figure 1 shows pictures of the surface wave launcher and the jig used in experiment to measure the channel matrix **H**. The images were taken to exemplify the setup at a much later stage than when the experiments were conducted. Hence, the wires are significantly less straight than they were in experiment where a lot of time was spent to make each wire as straight as possible.

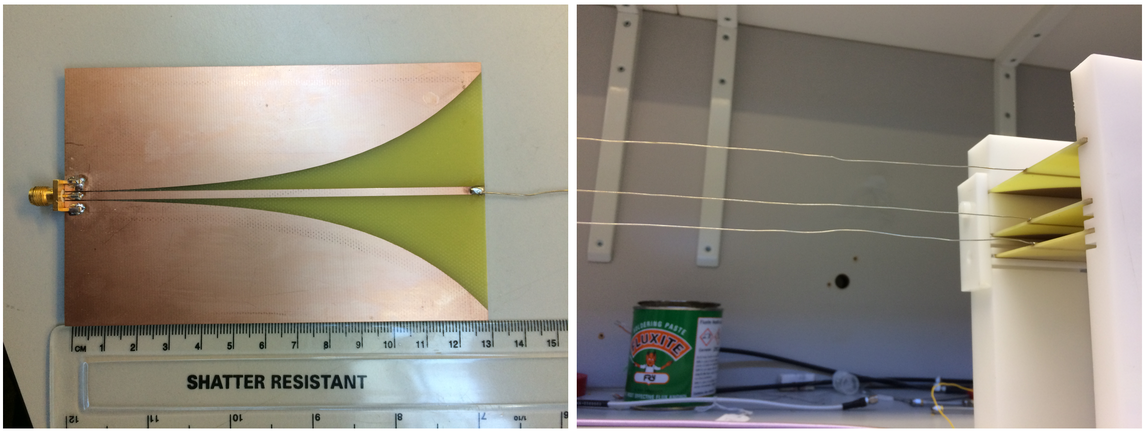


Figure 1: *Left:* Picture of the surface wave launcher. *Right:* Launchers in jig.

## 2 Imaginary Part of Eigenvectors

For completeness the imaginary parts of the measured eigenvectors of **H** for the two and three wire case are shown in Figure 2. As discussed in the main paper, the imaginary part in the two-wire case is generally small. A increase near 2.8 GHz is associated with a launcher induced resonance in experiment. In the three-wire case, the imaginary component increases with frequency as the setup size becomes comparable to the wavelength above around 1 GHz.

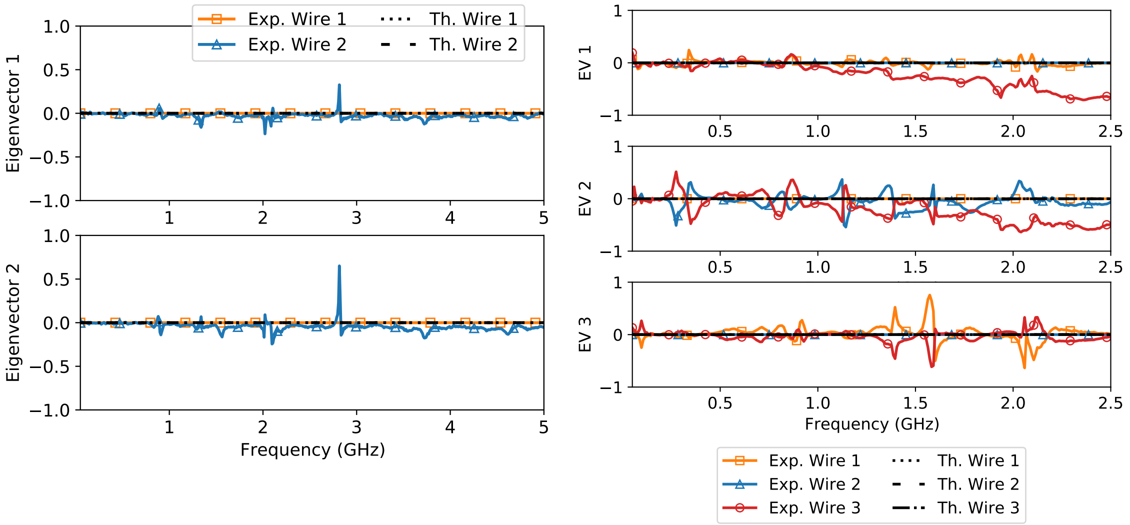


Figure 2: Imaginary part of the eigenvectors obtained theoretically (Th.) using the proposed MTL theory and experimentally (Exp.) via diagonalization of $\mathbf{H}$. *Left:* Two Wire Experiment. *Right:* Three Wire Setup
